# Supplementary material for: Recurrent Convolutions for Causal 3D CNNs
Source: arXiv:1811.07157 source file (2019-08-31)
Supplement: Supplementary file 1 [file supp_details.tex]

In this supplementary material, 
we first present a discussion Section~\ref{sec:discus}, 
followed by implementation details in Section~\ref{subsec:details}.
Next, we show a more in-depth analysis to understand the parameters of recurrent convolution in Section~\ref{sec:more}. 

\section{Discussion}\label{sec:discus}

\subsection{Effect of Weight Initialisation.}
Weights of inflated 2D layers in ResNet (base networks)~\cite{he2016deep} 
based I3D and our RCN networks 
are initialised with weights from a pre-trained ImageNet model train on RGB images.
In the case of RCN inflation in the third dimension is 1, 
practically, it is 2D weight matrix with the third dimension being 1.
As a result, we do need to replicate the weights like in the 3D layer of I3D.

Random initialisation for hidden state parameters resulted in suboptimal training. 
Thus, in all the experiments with RCN, we used identity matrix initialisation instead.
Here we show the result of training RCN with different initilisation of 
hidden-state $w_{hh}$ convolution and spatial $w_{xh}$ convolution in Table~\ref{table:hiddenInit}.
The first row of the table where both $w_{xh}$ and $w_{hh}$ of all the RCUs in 
RCN is initialised randomly using normal initialisation process described in~\cite{he2015delving}.

Table~\ref{table:hiddenInit} show the result of different initialisation of $w_{xh}$ and $w_{hh}$ 
respectively.
It is clear from the last row of the table that RCN performs best 
if $w_{xh}$ and $w_{hh}$ are initialised with ImageNet and identity matrix respectively.
It is noteworthy that the performance difference is relatively 
small in first three rows of that table as compared to the last row jump.

\begin{table}[t]
  %\vskip -3mm
  \centering
  {\footnotesize
  %\scalebox{0.95}
  {
  \begin{tabular}{cccc}
    \toprule
    $w_{xh}$ init & $w_{hh}$ init  & Clip-Acc\% & Video-Acc\%\\ %&Vid@Avg\\ 
    \midrule
    Random & Random  & 49.0 & 61.2 \\ 
    Random & Identity  & 49.3 & 61.8 \\ 
    ImageNet & Random    & 50.4 & 62.5 \\ 
    ImageNet & Identity  & \textbf{53.0} & \textbf{65.1} \\ 
    \bottomrule
  \end{tabular}
  }
  }
  \vspace{0.1cm}
  \caption{Video-level and clip-level action recognition accuracy on 
  the Kinetics validation set for different initilisation of 2D layer ($w_{xh}$) 
  and hidden state unit weights ($w_{hh}$) in RCU with ResNet-18-based RCN models 
  trained on 8 frame-long clip as an input. 
  These results were obtained using our older training setup, 
  which was is suboptimal than the current one presented in the main paper.
  The main difference is due to data, and number iterations have increased.}
  \label{table:hiddenInit} \vspace{-1mm}
\end{table}

\subsection{ImageNet initialisation} proves to be useful for both the I3D and our RCN models.
 While (2+1)D performs (Table~\ref{table:18results}, row 6) better than RCN (row 5) 
 with the random initialisation, our RCN recovers to improve over (2+1)D (row 6) 
 with ImageNet initialisation, whereas (2+1)D cannot make use of free ImageNet initialisation.
 This seems to be a severe drawback for the (2+1)D model, and a big advantage for I3D and RCN.
 One may argue that, if the purpose is to build on existing 2D models, then RCN and I3D are a better choice, 
 whereas if new 3D models are preferred then (2+1)D might prove useful. 
 The latter does provide better performance with the random initialisation, 
 but at the price of requiring many more parameters than RCN.

% \vspace{1mm}
% \noindent
% \textbf{Random initialisation} for hidden state parameters resulted in unstable training. Thus,
% in all the experiments with RCN, we used identity matrix initialisation instead.
% Identity matrix initialisation helps to capture forget capabilities as well, 
% as suggested by~\cite{le2015simple}.
% An ablation study on the effect of initialisation is provided in the supplementary material.
%This is evident in our experiments on the very long MultiThumos videos (\S~\ref{subsec:multithumos}).

\subsection{On Input Clip Length} 
Input clip length is another factor in determining the final performance of any network. 
We can see from the Table that all the Inception-based models are trained on 64 frame-long clips, one of the reasons why Inception nets work better that ResNet models while using fewer parameters. Among the latter, ResNet101-I3D-NL~\cite{nonlocal2018wang} is shown to work better with an even longer input clip length. 
%This gain, however, comes with a tweaking of the training process -- e.g.,  Wang~\etal~\cite{nonlocal2018wang} initialise from pre-trained 32 frame-clip models and turn-off the batch normalisation layers. 
Thus, the evidence supports that training on larger input sequences boosts performance while clashing with memory limitations. 

In our experiments, as mentioned, we stuck to 8 or 16 frame clips as input and compared our proposed RCN with baseline I3D models.
We think this provides enough evidence of the validity of our proposal to move away from 
temporal convolutional networks~\cite{xie2018rethinking,nonlocal2018wang,tran2018closer,carreira2017quo}, and replace them with more sophisticated \emph{and} causal structures.
As with the role of additional layers, it is fair to predict that more extensive training on more extended clips (32,64,128) has a serious potential to take RCN to outperform state of the art in absolute terms.

\subsection{On the Efficient Training of 3D Networks}
Two basic things are clear from our experience with training heavy 3D models (I3D, (2+1)D, RCN) on large-scale datasets such as Kinetics.
Firstly, training is very computationally expensive and memory bulky; secondly, longer input clips are crucial to achieving better optimisation which, however, renders the first issue even more severe. 
We feel that how to train these model efficiently is still a wide-open problem, whose solution is essential to speed up the process for broader adoption.
We observed that ImageNet initialisation does speed up the training procedure, and helps reach local minima much quicker.
In the case of both I3D and RCN, ImageNet initialisation improves the video classification accuracy on  
Kinetics by almost $3\%$ compared to random initialisation when using the same number of training iterations, 
as shown in the first and last row of Table~\ref{table:hiddenInit}.
% Furthermore, 16 frames models also exhibit an almost $3\%$ performance improvement compared to the corresponding 8 frame models, but this comes at nearly twice the computational cost.

The bottom line is that we should strive for more efficient implementations of 3D models for the sake of their adoption. % Fabio is not that obvious?

\section{Implementation Details}\label{subsec:details}
All models with $8$ and $16$ long clip as input are trained with batch size of 
$64$ and $32$ respectively.
%and models with $16$ frame long clip are trained with batch $$
We used maximum for four 1080Ti GPUs (11GB VRAM each) while training all the models.
We used Pytorch library to implement all of the models from scratch, 
and we used the ResNet architecture of 
2D model from pytorch library's 
model zoo\footnote{https://github.com/pytorch/vision/tree/master/torchvision/models}.

\textbf{Input Data Preparations.}
We apply the same set of input data transformations to each frame in an input clip.
Data agumentation transformations include random crop, radom horizontal flip, affine transformations, and temporal jittering.

\section{Hidden State Parameters}~\label{sec:more}
Figure~\ref{fig:statsRandInits08} show the mean and 
standard deviation (Std) of weight matrixes ($w_{hh}$) 
of the hidden state at every RCU layer in our RCN network. 
We see the drop in standard deviation across different models 
(ResNet-18 in Figure~\ref{fig:statsRandInits08} and ResNet-34 in Figure~\ref{fig:statsRandInits16}(b))
 and different input clip-lengths used for training 
((8 in Figure~\ref{fig:statsRandInits08} and 16 in Figure~\ref{fig:statsRandInits16}(b))).
The drop in standard deviation and an increase in mean values of diagonal values means towards sparsity.
The increase in sparsity with depth increase can also be observed in the Figure~\ref{fig:heatmaps}, especially in the last layer (Layer 16), elements on diagonal have higher weights, and the first layer (Layer 1) has higher values distribute all around in the matrix.

We can conclude the increase in sparsity increases focuses on diagonal elements, hence, the same feature 
focus more on the time dimension of the same feature than other features from the previous hidden-state.
It is a reasonable explanation because we expect the network to learn from the different feature at small depth-level and focus more on same feature (i.e. focus on time aspect of the same feature) more with the increase in the depth-level.

\noindent
\textbf{Acknowledgement:} This work was partly supported by the European Union's Horizon 2020 research and innovation programme under grant agreement No. 779813 (SARAS).

\begin{figure*}[t]
  \centering
  \includegraphics[scale=0.50]{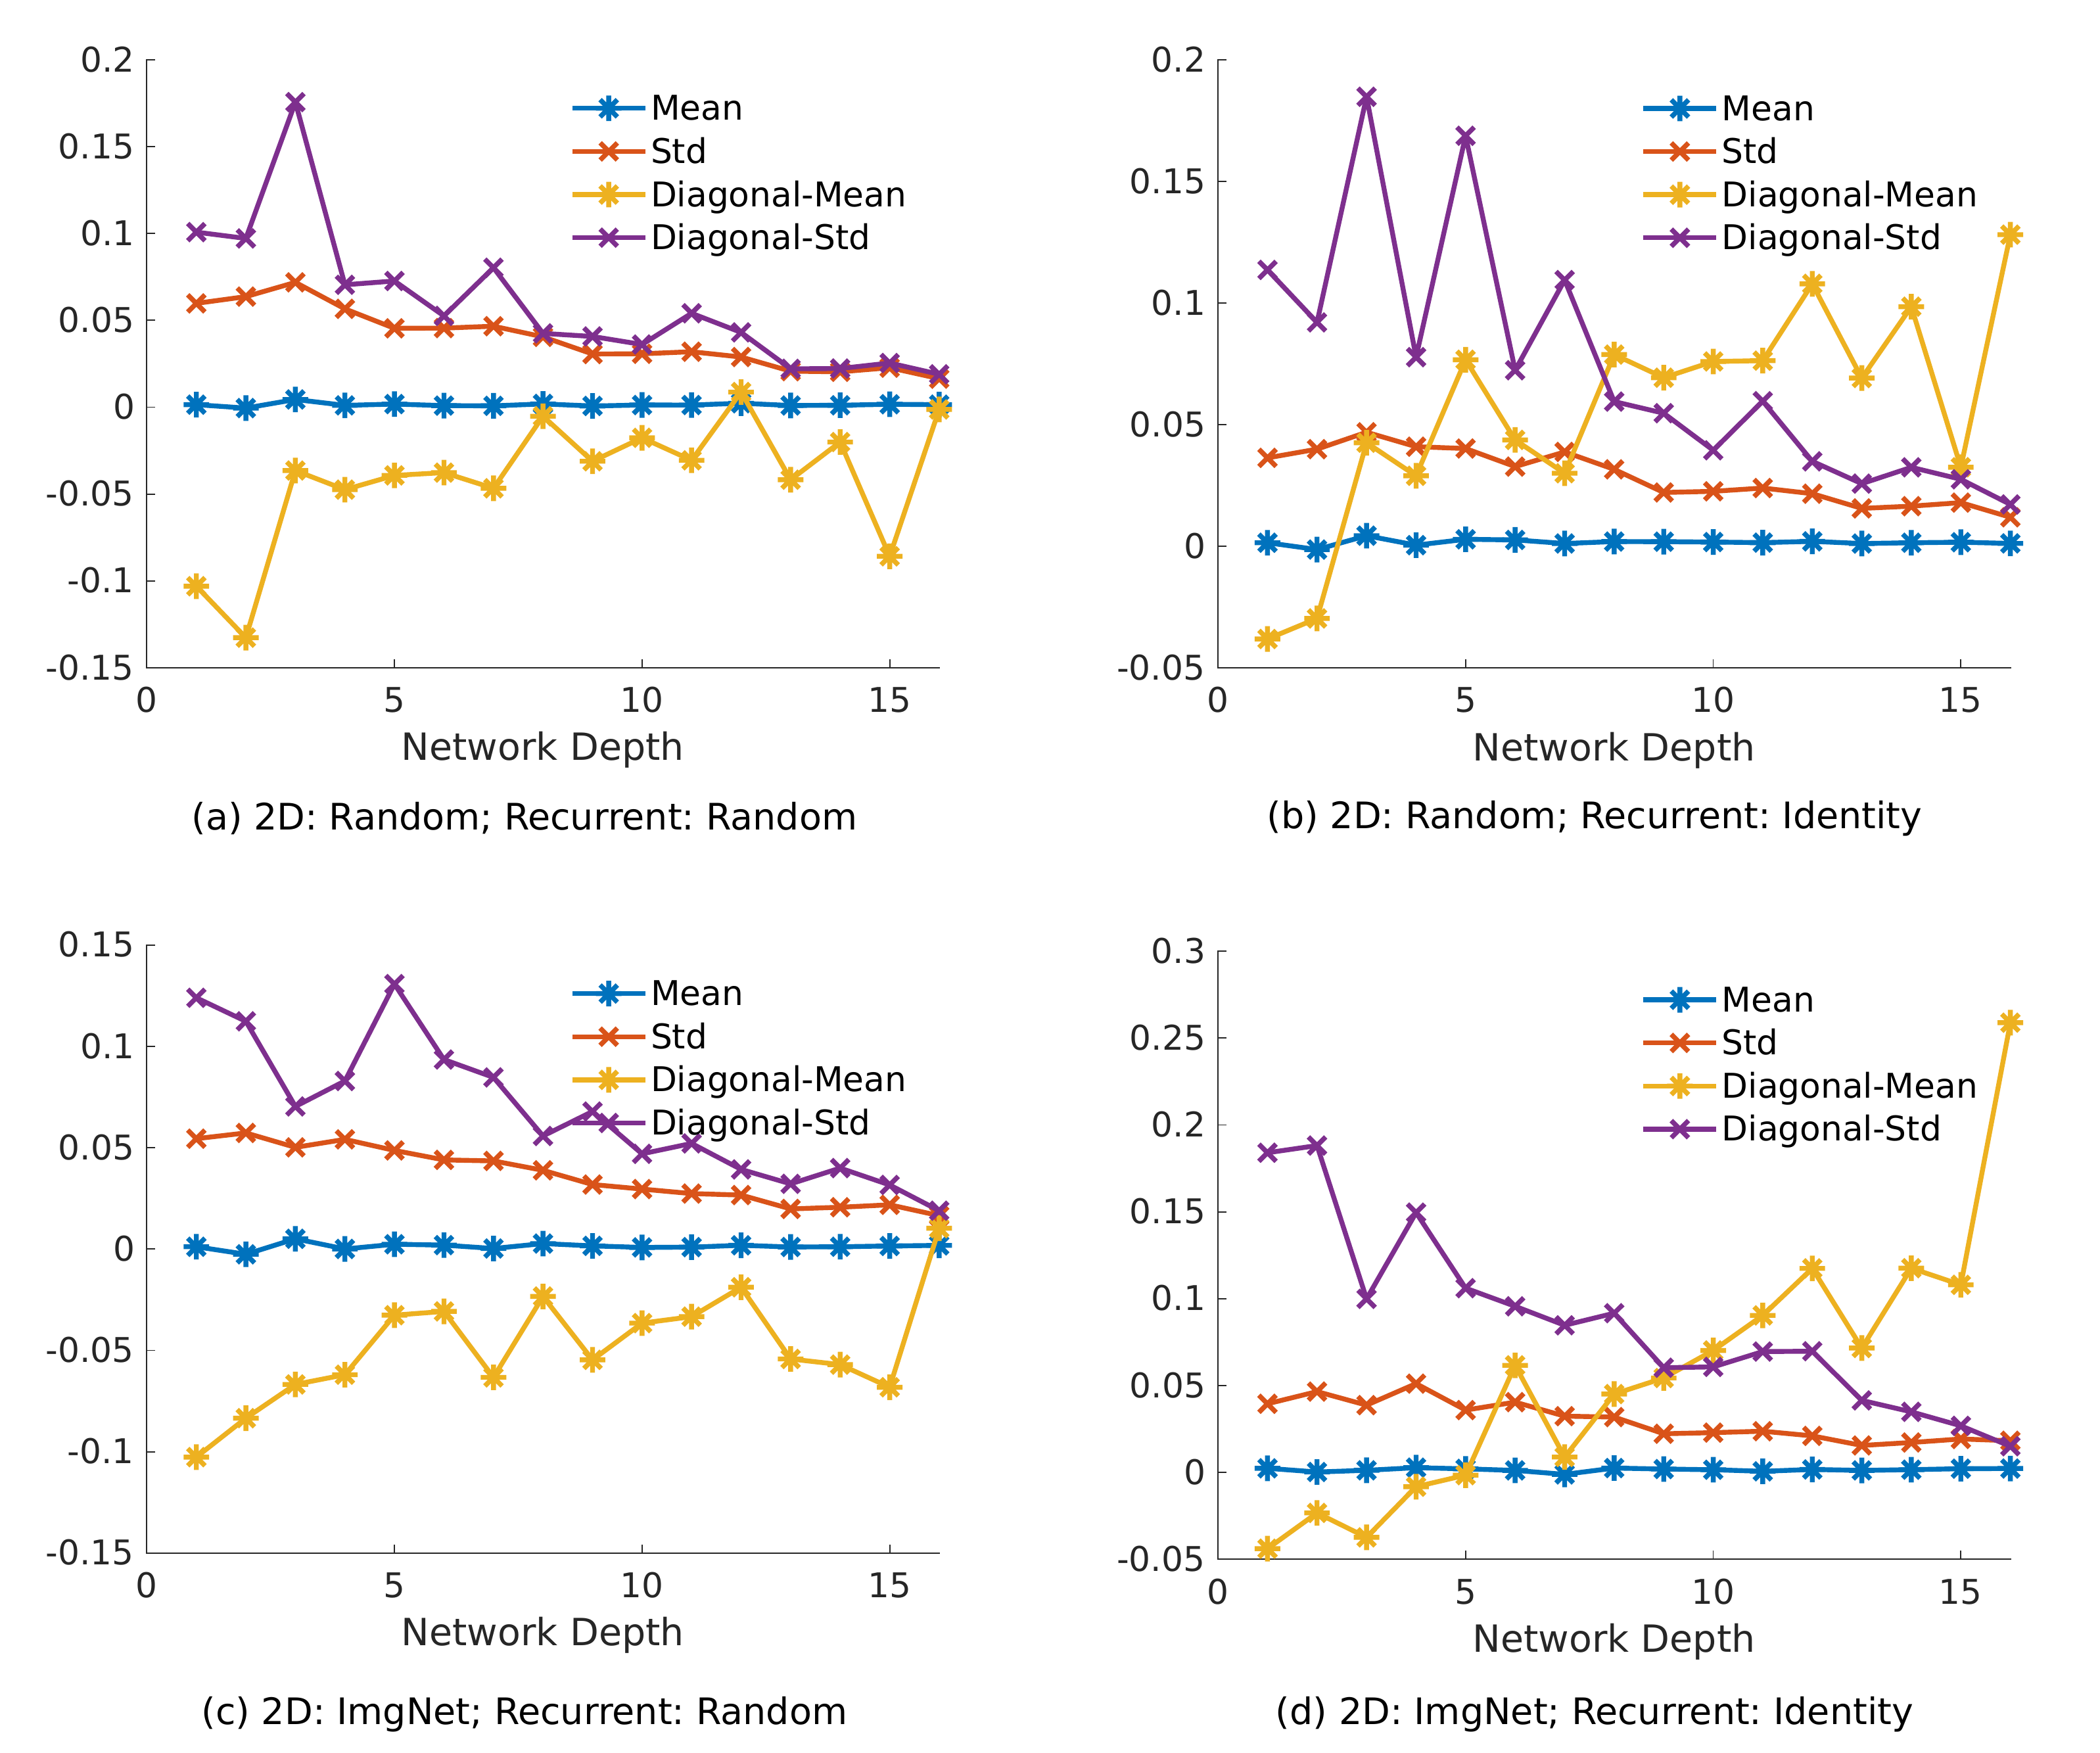}
  \caption{Mean and standard deviation (Std) of weight matrixes ($w_{hh}$) 
      of the hidden state at every RCU layer in the network based on ResNet-18, 
      along with the mean, and Std of diagonal elements. 
      Networks are trained on an input clip-length of 8.}
\label{fig:statsRandInits08}
\end{figure*}

\begin{figure*}[t]
  \centering
  \includegraphics[scale=0.50]{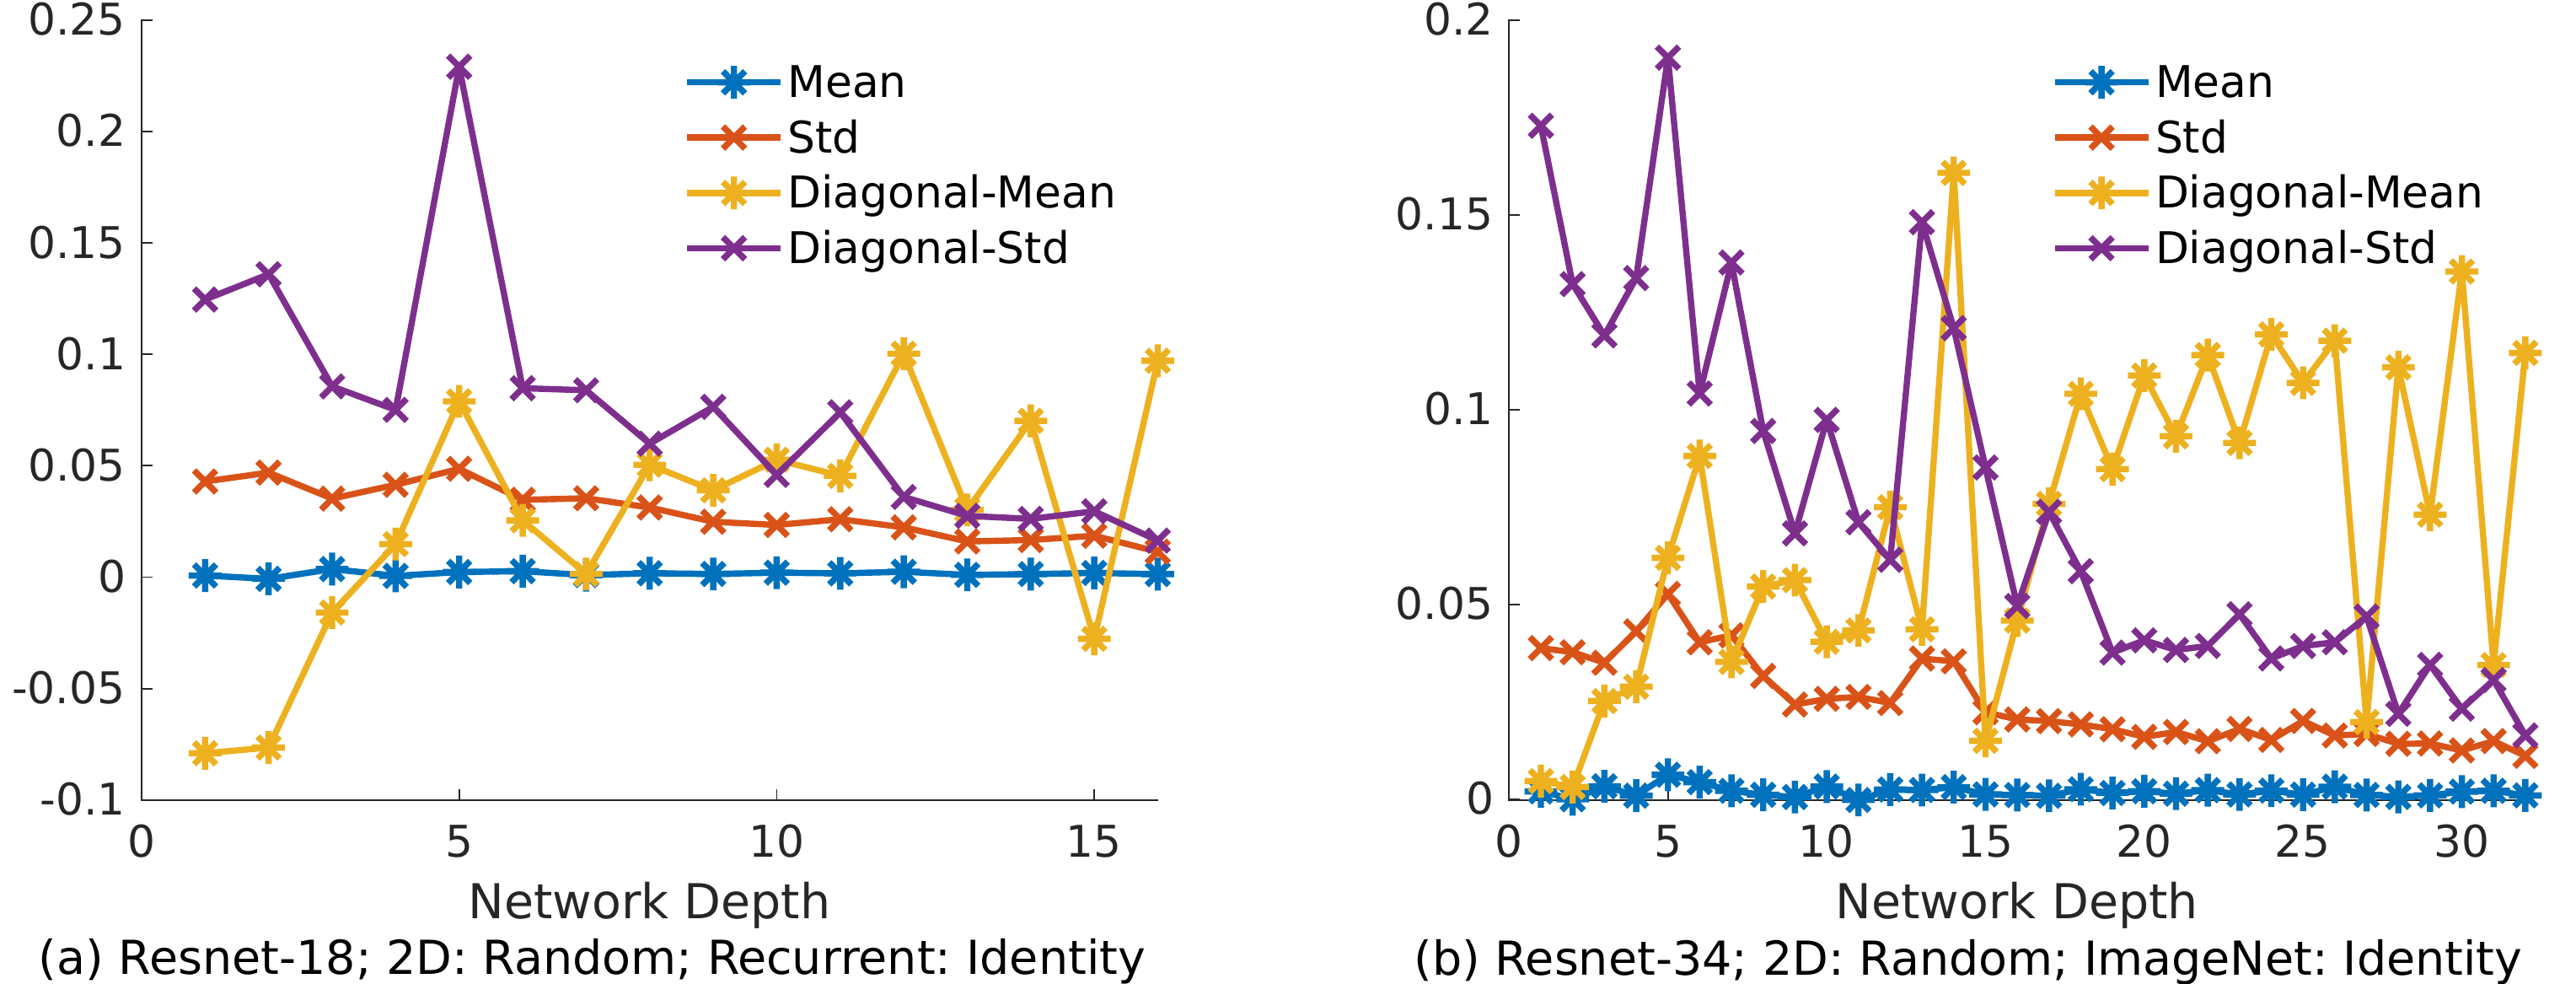}
  \caption{Mean and standard deviation (Std) of weight matrixes ($w_{hh}$) 
      of the hidden state at every RCU layer in the network based on ResNet-18 (a) and ResNet-34 (b), 
      along with the mean, and Std of diagonal elements. 
      Networks are trained on an input clip-length of 16.}
\label{fig:statsRandInits16}
\end{figure*}

\begin{figure*}[t]
  \centering
  \includegraphics[scale=0.5]{figures/mats.pdf}
  \caption{Heat map of weight matrixes ($w_{hh}$) 
      of the hidden state at every RCU layer in the network based on ResNet-18.
      Parula colourmap (from matlab) is used, 
      where blue is smallest values and yellow is the highest i.e. dark to bright.}
\label{fig:heatmaps}
\end{figure*}
